# Supplementary material for: Is Everything in Order? A Simple Way to Order Sentences
Source: arXiv:2104.07064 source file (2021-09-17)
Supplement: Supplementary file 1 [file appendix.tex]

% \documentclass[11pt]{article}

% % Remove the "review" option to generate the final version.
% \usepackage[review]{emnlp2021}
% % \usepackage{emnlp2021}

% % Standard package includes
% \usepackage{times}
% \usepackage{latexsym}

% % For proper rendering and hyphenation of words containing Latin characters (including in bib files)
% \usepackage[T1]{fontenc}
% % For Vietnamese characters
% % \usepackage[T5]{fontenc}
% % See https://www.latex-project.org/help/documentation/encguide.pdf for other character sets

% % This assumes your files are encoded as UTF8
% \usepackage[utf8]{inputenc}


% % If the title and author information does not fit in the area allocated, uncomment the following
% %
% %\setlength\titlebox{<dim>}
% %
% % and set <dim> to something 5cm or larger.

% % \documentclass[11pt,a4paper]{article}
% % \usepackage[hyperref]{emnlp2021}
% % \usepackage{times}
% % \usepackage{latexsym}
% % \renewcommand{\UrlFont}{\ttfamily\small}

% % This is not strictly necessary, and may be commented out,
% % but it will improve the layout of the manuscript,
% % and will typically save some space.
% \usepackage{microtype}
% \usepackage{natbib}
% % \usepackage{subfigure}
% \usepackage{caption}

% % \aclfinalcopy % Uncomment this line for the final submission
% %\def\aclpaperid{***} %  Enter the acl Paper ID here

% %\setlength\titlebox{5cm}
% % You can expand the titlebox if you need extra space
% % to show all the authors. Please do not make the titlebox
% % smaller than 5cm (the original size); we will check this
% % in the camera-ready version and ask you to change it back.


% \include{preamble}
% \usepackage{setspace}
% \usepackage[a4paper]{geometry}
% \usepackage{titlesec}
% \usepackage{amssymb}
% \usepackage{mathtools}
% \usepackage{lipsum}

% \usepackage{amsmath}

% \usepackage{multirow}      
% \usepackage{multicol}
% \usepackage{pgfplots}
% \pgfplotsset{compat=1.17}


% \newcommand\BibTeX{B\textsc{ib}\TeX}
% \newcommand\Tstrut{\rule{0pt}{2.6ex}}       % "top" strut
% \newcommand\Bstrut{\rule[-0.9ex]{0pt}{0pt}} % "bottom" strut
% \newcommand{\TBstrut}{\Tstrut\Bstrut} % top&bottom struts


% % our packages
% \usepackage[normalem]{ulem}
% \usepackage{comment}
% \usepackage{blindtext, subfig} 
% \usepackage[linecolor=orange]{todonotes}
% \usepackage{hhline}
% \usepackage{booktabs} % To thicken table lines
% \usepackage{enumitem}% to reduce space between items.


% \newcommand{\fb}[1]{\textcolor{blue}{Faeze: #1}}
% \newcommand{\SC}[1]{\todo[color=cyan!40]{\footnotesize SC: #1}}
% % \newcommand{\sbrc}[1]{\textcolor{purple}{Somnath: #1}}
% \newcommand{\sbrc}[1]{\todo[color=red!40]{\footnotesize #1}}


% \newcommand{\rebart}{\textsc{Re}-\textsc{Bart}\xspace}

% \newcommand{\fbb}[1]{\todo[color=green!40]{\footnotesize #1}}


% \title{Supplementary Material for the paper titled: \\ \emph{Is Everything in Order?} A Simple Way to Order Sentences}

% % \author{First Author \\
% %   Affiliation / Address line 1 \\
% %   Affiliation / Address line 2 \\
% %   Affiliation / Address line 3 \\
% %   {\tt email@domain} \\\And
% %   Second Author \\
% %   Affiliation / Address line 1 \\
% %   Affiliation / Address line 2 \\
% %   Affiliation / Address line 3 \\
% %   {\tt email@domain} \\}

% \date{}

% \begin{document}
% \maketitle
% \section{Implementation Details}


% \section{Analysis}
% \label{sec:appendix}
%%% moved to main body
% \subsection{Prediction Displacement}

% For instances where the model prediction was wrong $Y \neq Y^*$, we investigate how far was the model prediction $Y$ was from the gold label $Y^{*}$. To evaluate this we compute $d(Y, Y^*)$, the minimum number of swaps required to retrieve $Y^*$ from $Y$. We experiment on Wikipedia Movie Plots dataset where the performance of Reorder-BART was not as good as other datasets. From Figure~\ref{fig:var-acc-dyy}, we observe that most of the incorrectly predicted samples had a low $d_{s}(Y, Y^*)$, with 70\% of the incorrect predictions having $d(Y, Y^*) \leq 6$. This shows that even if the model make a wrong prediction, it mostly misses a few positions and does not get the entire order wrong. %\SC{Why is accuracy not measuring this phenomenon?} \sbrc{it does but I feel quantization of accuracy is not every elegant, which $d_{s}(Y, Y^*)$ handles better} \SC{You need to justify defining a new measure in the text. }


% \begin{figure}[h!]
%     \centering
%     \input{paper/figures/degree_correctly_predicted}
%     \caption{\small Plot shows how many instances were incorrectly predicted for each $d(Y, Y^*)$ for Wikipedia Movie Plots.}
%     \label{fig:var-acc-dyy}
% \end{figure}




% \end{document}
